# Supplementary material for: Laser intracavity absorption magnetometry for optical quantum sensing
Source: arXiv:2512.24951 source file (2026-08-28)
Supplement: Supplementary file 2 [file preambel_sup.tex]

\usepackage{graphicx}
\usepackage[usenames,dvipsnames]{xcolor}
\usepackage{amssymb,amsfonts,amsmath}
\usepackage[colorlinks=true,citecolor=Cerulean,linkcolor=RubineRed,urlcolor=Cerulean]{hyperref}
\usepackage{epstopdf}
\usepackage{bm}
\usepackage{bbold}
\usepackage{upgreek}
\usepackage[inline]{enumitem}
\usepackage{booktabs}
\usepackage{multirow}
\usepackage[normalem]{ulem}
\usepackage{IEEEtrantools}
\usepackage{subfigure}
\usepackage{subcaption}

% CGT
\usepackage{float}
%\usepackage{multicol}

\usepackage{afterpage}
\newcommand\blankpage{%
    \null
    \thispagestyle{empty}%
    \addtocounter{page}{-1}%
    \newpage}

\usepackage{verbatim}
\newcommand{\detailtexcount}[1]{%
  \immediate\write18{texcount -merge -sum -q #1.tex output.bbl > #1.wcdetail }%
  \verbatiminput{#1.wcdetail}%
}
\newcommand{\quickwordcount}[1]{%
  \immediate\write18{texcount -1 -sum -merge -q #1.tex output.bbl > #1-words.sum }%
  \input{#1-words.sum} words%
}
\newcommand{\quickcharcount}[1]{%
  \immediate\write18{texcount -1 -sum -merge -char -q #1.tex output.bbl > #1-chars.sum }%
  \input{#1-chars.sum} characters (not including spaces)%
}
\usepackage{lipsum, babel}
\usepackage{sidecap}
\usepackage{hyperref}
\hypersetup{
    colorlinks=true,
    linkcolor=magenta,%blue,
    filecolor=magenta,      
    urlcolor=cyan,
    pdftitle={Overleaf Example},
    pdfpagemode=FullScreen,
    }
\usepackage{xr}
\makeatletter
\newcommand*{\addFileDependency}[1]{% argument=file name and extension
  \typeout{(#1)}
  \@addtofilelist{#1}
  \IfFileExists{#1}{}{\typeout{No file #1.}}
}
\makeatother

\newcommand*{\myexternaldocument}[1]{%
    \externaldocument{#1}%
    \addFileDependency{#1.tex}%
    \addFileDependency{#1.aux}%
}

% maths commands
\newcommand{\im}{\mathrm{i}}
\newcommand{\kBT}{k_\mathrm{B}T}
\newcommand{\kB}{k_\mathrm{B}}
\newcommand{\ud}{\mathrm{d}}
\newcommand{\bv}[1]{{\boldsymbol #1}}
\newcommand{\ket}[1]{\left|#1\right\rangle}
\newcommand{\bra}[1]{\left\langle #1\right|}
\newcommand{\ketbra}[2]{\left|#1\right\rangle \left\langle #2 \right|}
\renewcommand{\vec}[1]{{\bm #1}}
\newcommand{\gtwo}{\textsl{g}^2}
\newcommand{\EXP}[1]{~\times~10^{#1}}
\newcommand{\Ang}{${\rm \AA ngstr\ddot{o}m}$}


% filled and empty circles
\usepackage{txfonts}
\usepackage{latexsym}

% typsetting helpers
\newcommand{\tosupp}[1]{{\color{ForestGreen}{\bf SUPP}: {\em #1}}}
\newcommand{\tocut}[1]{{\color{BrickRed}{\bf CUT}: \sout{#1}}}
\newcommand{\todo}[1]{{\color{DarkOrchid} $\{\{${\bf TODO}: #1$\}\}$}}
\newcommand{\jhdm}[1]{{\color{PineGreen}$\langle\langle$#1$\rangle\rangle$}}
\newcommand{\cgt}[1]{{\color{RedOrange}#1}}
\newcommand{\gp}[1]{{\color{NavyBlue}#1}}
\newcommand{\ts}[1]{{\color{Lavender}#1}}
% compiling options
\graphicspath{ {./figz/} }
\bibliographystyle{apsrev4-2}


\newlist{custominlist}{enumerate*}{1}
\setlist[custominlist]{label=(\roman*)}%, before=\unskip{: }, itemjoin={{; }}, itemjoin*={{, and }}}

\makeatletter
\newcommand{\makesupplementarytitle}{
  \clearpage
  \onecolumngrid
  \begin{center}
    \begingroup
      \parindent=0pt
      \renewcommand\baselinestretch{1.1}%
      {\large\bfseries Supplementary Information\par}
    \endgroup
  \end{center}
  \vspace{2em}
  \twocolumngrid
}
\makeatother
